# Supplementary material for: Graph Neural Networks for Decentralized Multi-Robot Path Planning
Source: arXiv:1912.06095 source file (2020-07-14)
Supplement: Supplementary file 1 [file appendix.tex]

\section{Supplementary Results}
\label{sec:Appendix}
This appendix presents supplementary material for our approach.
Fig.~\ref{fig:demo} exemplifies a typical failure case caused by inter-robot collision (i.e., in this case, a position-swap). 
Fig.~\ref{fig:results_generalization_impact_OE_K2} compares the GNN performance with and without the online expert (OE). We also investigate the impact of filter taps $K$ (Fig.~\ref{fig:results_generalization_impact_K}).

% Fernando:
%1) State the objective: to compare the GNN without OE with the one with OE. And to compare for different K's. ONE PARAGRAPH.
%2) Re-state what the experiment setting is: how many you trained on, what architectures, etc. ONE PARAGRAPH.
%3) Explain in detail the figures. One figure per paragraph, two or three sentences per paragraph. ONE PARAGRAPH PER FIGURE. (You can join one paragraph per two figures, if you prefer)

Fig.~\ref{fig:demo} illustrates the target path computed by the expert algorithm and the path computed by the network trained and tested on 8 robots. Different from a search-based method, the proposed framework can not explore the future collision ahead of time. This results in the inter-robot collision in Fig.~\ref{fig:demo} (b). Although the collision shielding can force robots to remain idle, the lack of solutions for such scenarios (e.g., position-swap) in the offline data-set causes the deadlock. This yields the need for an online expert (through a data-set aggregation method, as described in Sec.~\ref{subsec:online_Expert}) that provides a solution from this configuration onward.

\begin{figure}[tb]
    \centering
    \begin{subfigure}[t]{0.28\columnwidth}
        \centering
        \frame{\includegraphics[height=3cm]{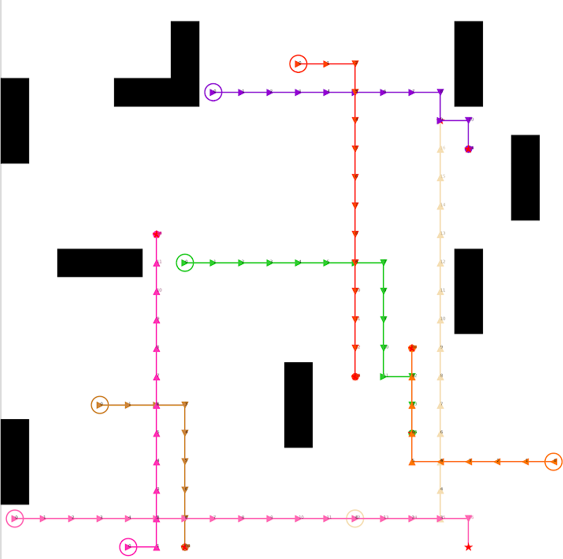}}
        \caption{Target path}
    \end{subfigure}
        \begin{subfigure}[t]{0.7\columnwidth}
        \centering
        \includegraphics[height=3.05cm]{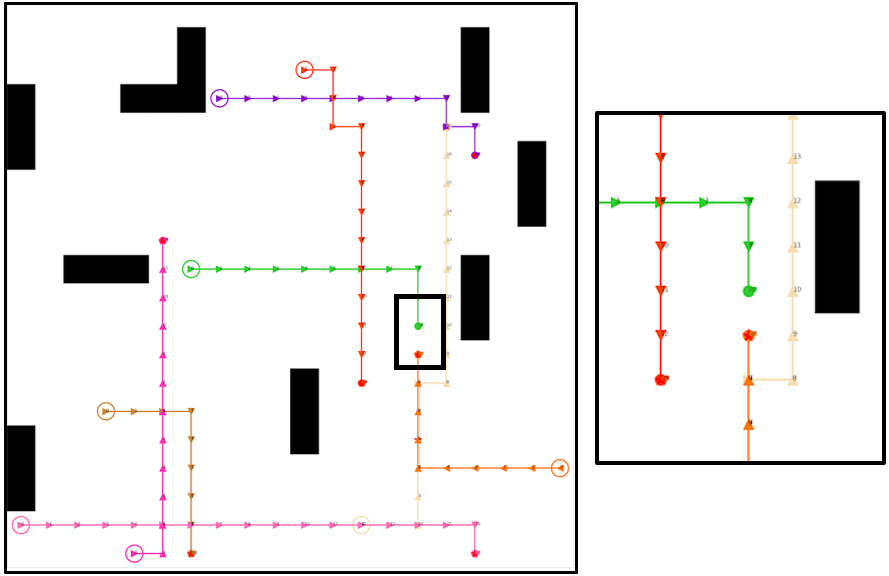}
        \caption{Predicted path}
    \end{subfigure}
    \caption{\normalfont Demo of the path of individual robots. Panel (a) illustrates the target path of expert algorithm,and Panel (b) illustrates the predicted path from the network without online expert is trained and tested on 8 robots. Note that, the deadlock caused by collision shielding is zoom in aside(b).}
    \label{fig:demo}
\end{figure}

To further evaluate the improvement provided by the online expert, we trained the GNN with and without the online expert, and tested the networks on 16 and 32 robots in $28 \times 28$ and $40\times40$ environments. Fig.~\ref{fig:results_generalization_impact_OE_K2} shows a distribution shift from the GNN without the online expert to the GNN with the online expert. We see how the GNN network with the online expert tends to generalize better than the one without, since the proportion of robots reaching the goal is significantly larger. This holds for tests on 16 and 32 robots, indicating the network starts to learn how to solve those cases that the GNN network without the online expert could not solve.

To evaluate the impact of filter taps ($K$), we increases the hop count $K$ from 2 into 3 in our experiment of testing 20 and 40 robots. We observed the proportion of robots reaching the goal slightly increases from $K=2 $ into $3$ in Fig.~\ref{fig:results_generalization_impact_K}. 

\begin{figure}[tb]
    \centering
    \begin{subfigure}[t]{0.48\columnwidth}
        \centering
        \includegraphics[width=\columnwidth]{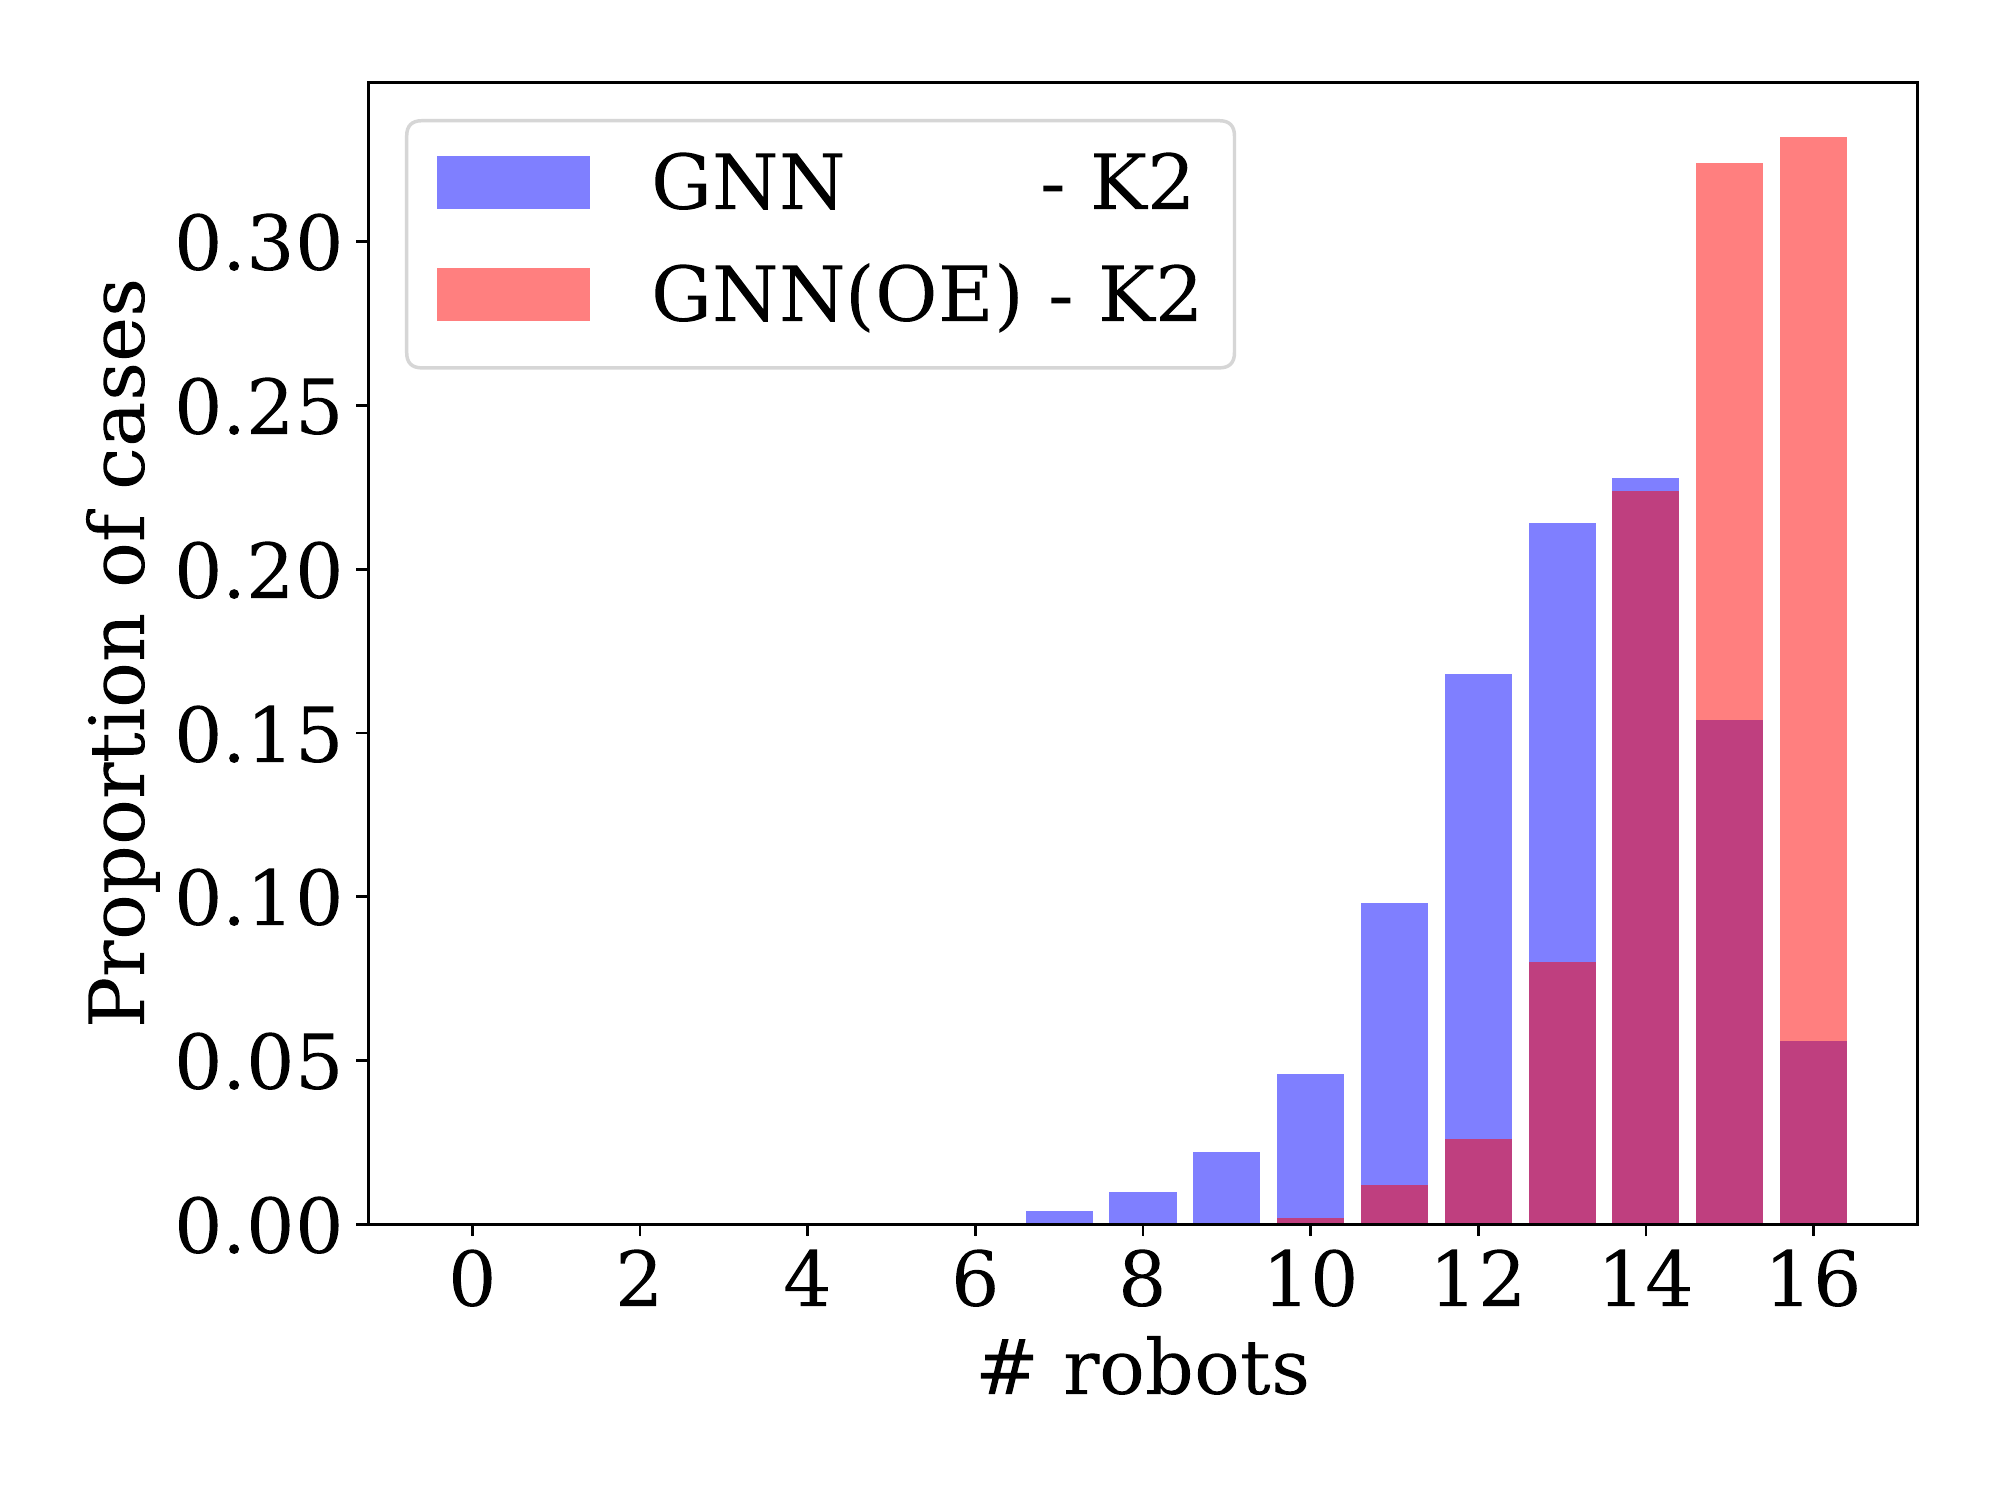}
        \caption{Tested on 16 robots}
    \end{subfigure}
        \begin{subfigure}[t]{0.48\columnwidth}
        \centering
        \includegraphics[width=\columnwidth]{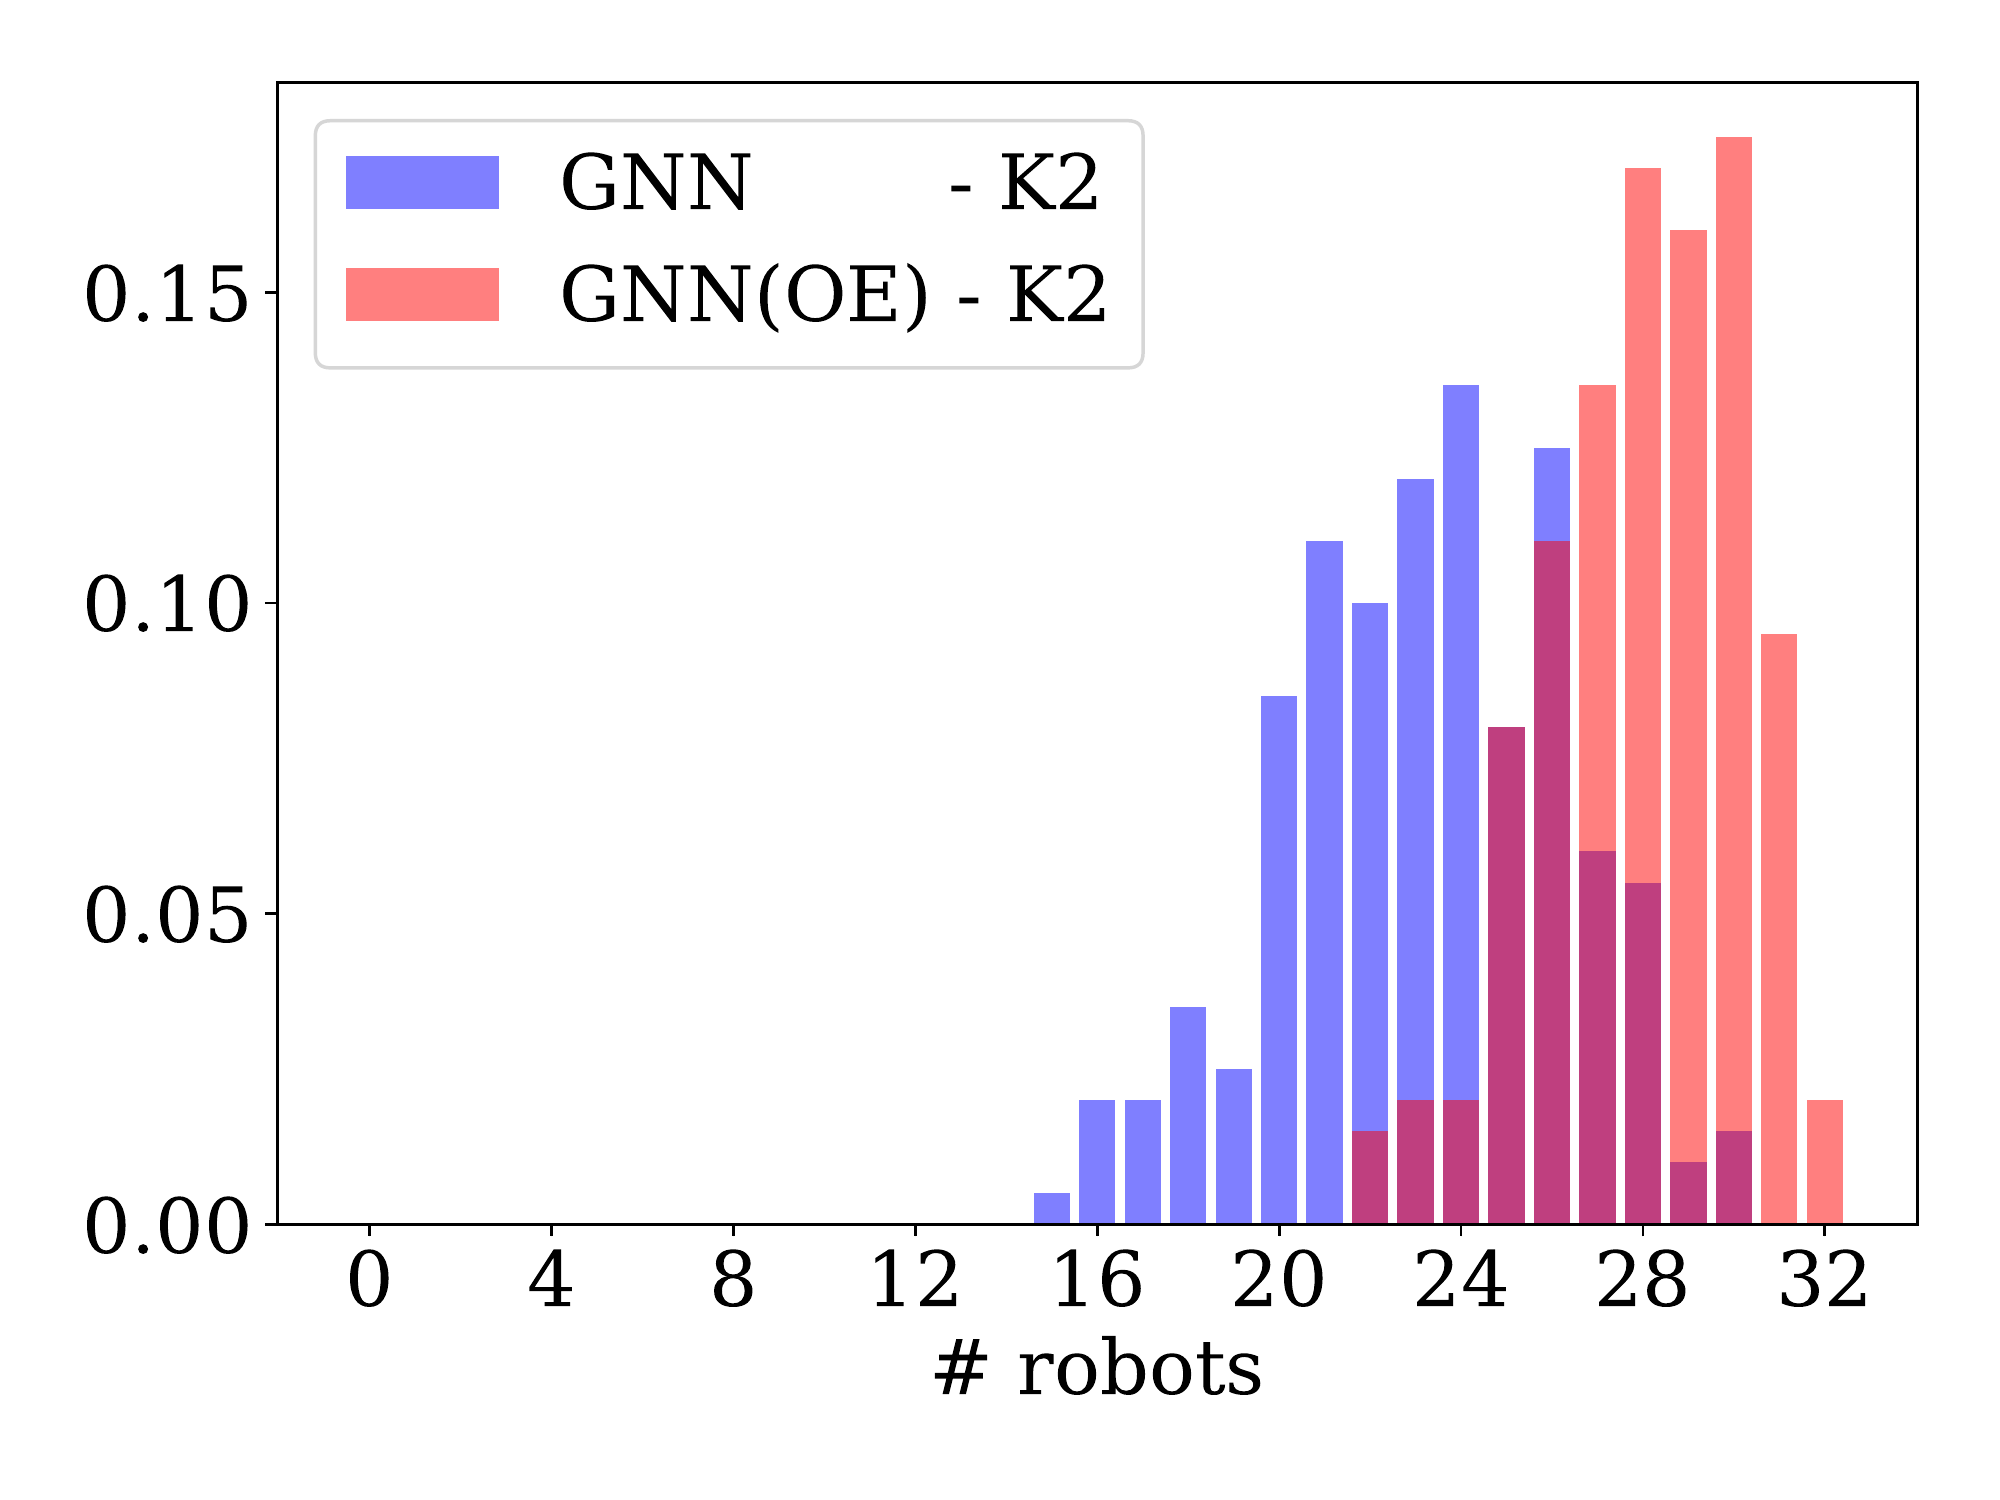}
        \caption{Tested on 32 robots}
    \end{subfigure}
    \caption{\normalfont Histogram of proportion of cases distributed over the number of robots reaching their goal; the network is trained on 8 robots and tested on 16 robots in (a), and tested on 32 robots in (b). Panels (a) and (b) use hop count $K=2$ without and with online expert, respectively.}
    \label{fig:results_generalization_impact_OE_K2}
\end{figure}

\begin{figure}[tb]
    \centering
    \begin{subfigure}[t]{0.48\columnwidth}
        \centering
        \includegraphics[width=\columnwidth]{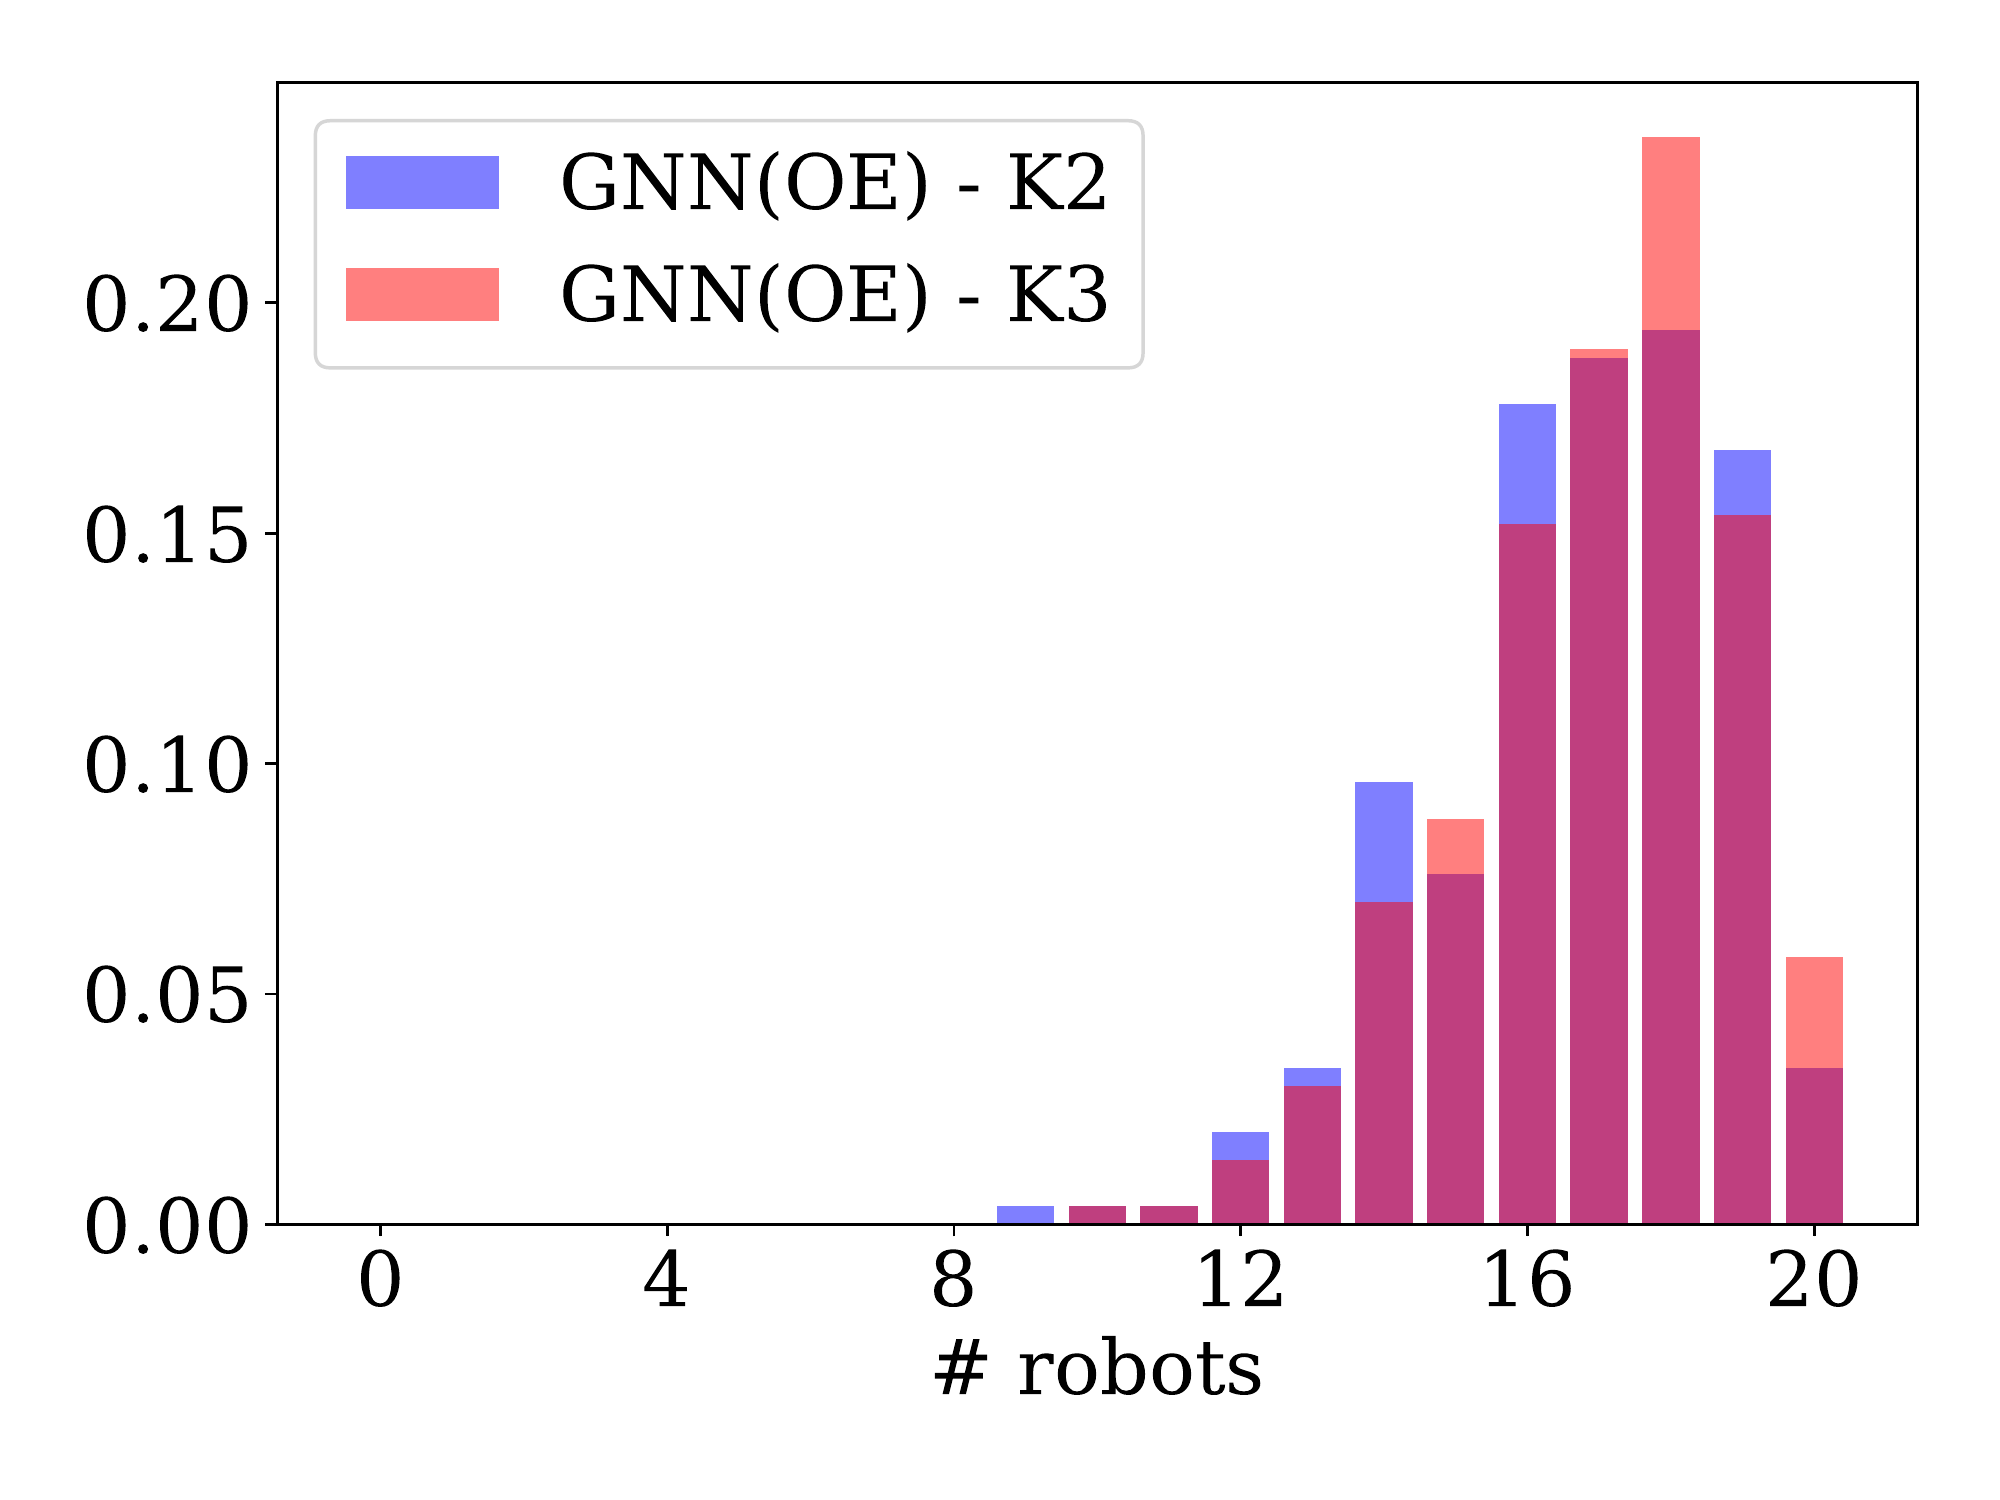}
        \caption{Tested on 20 robots}
    \end{subfigure}
        \begin{subfigure}[t]{0.48\columnwidth}
        \centering
        \includegraphics[width=\columnwidth]{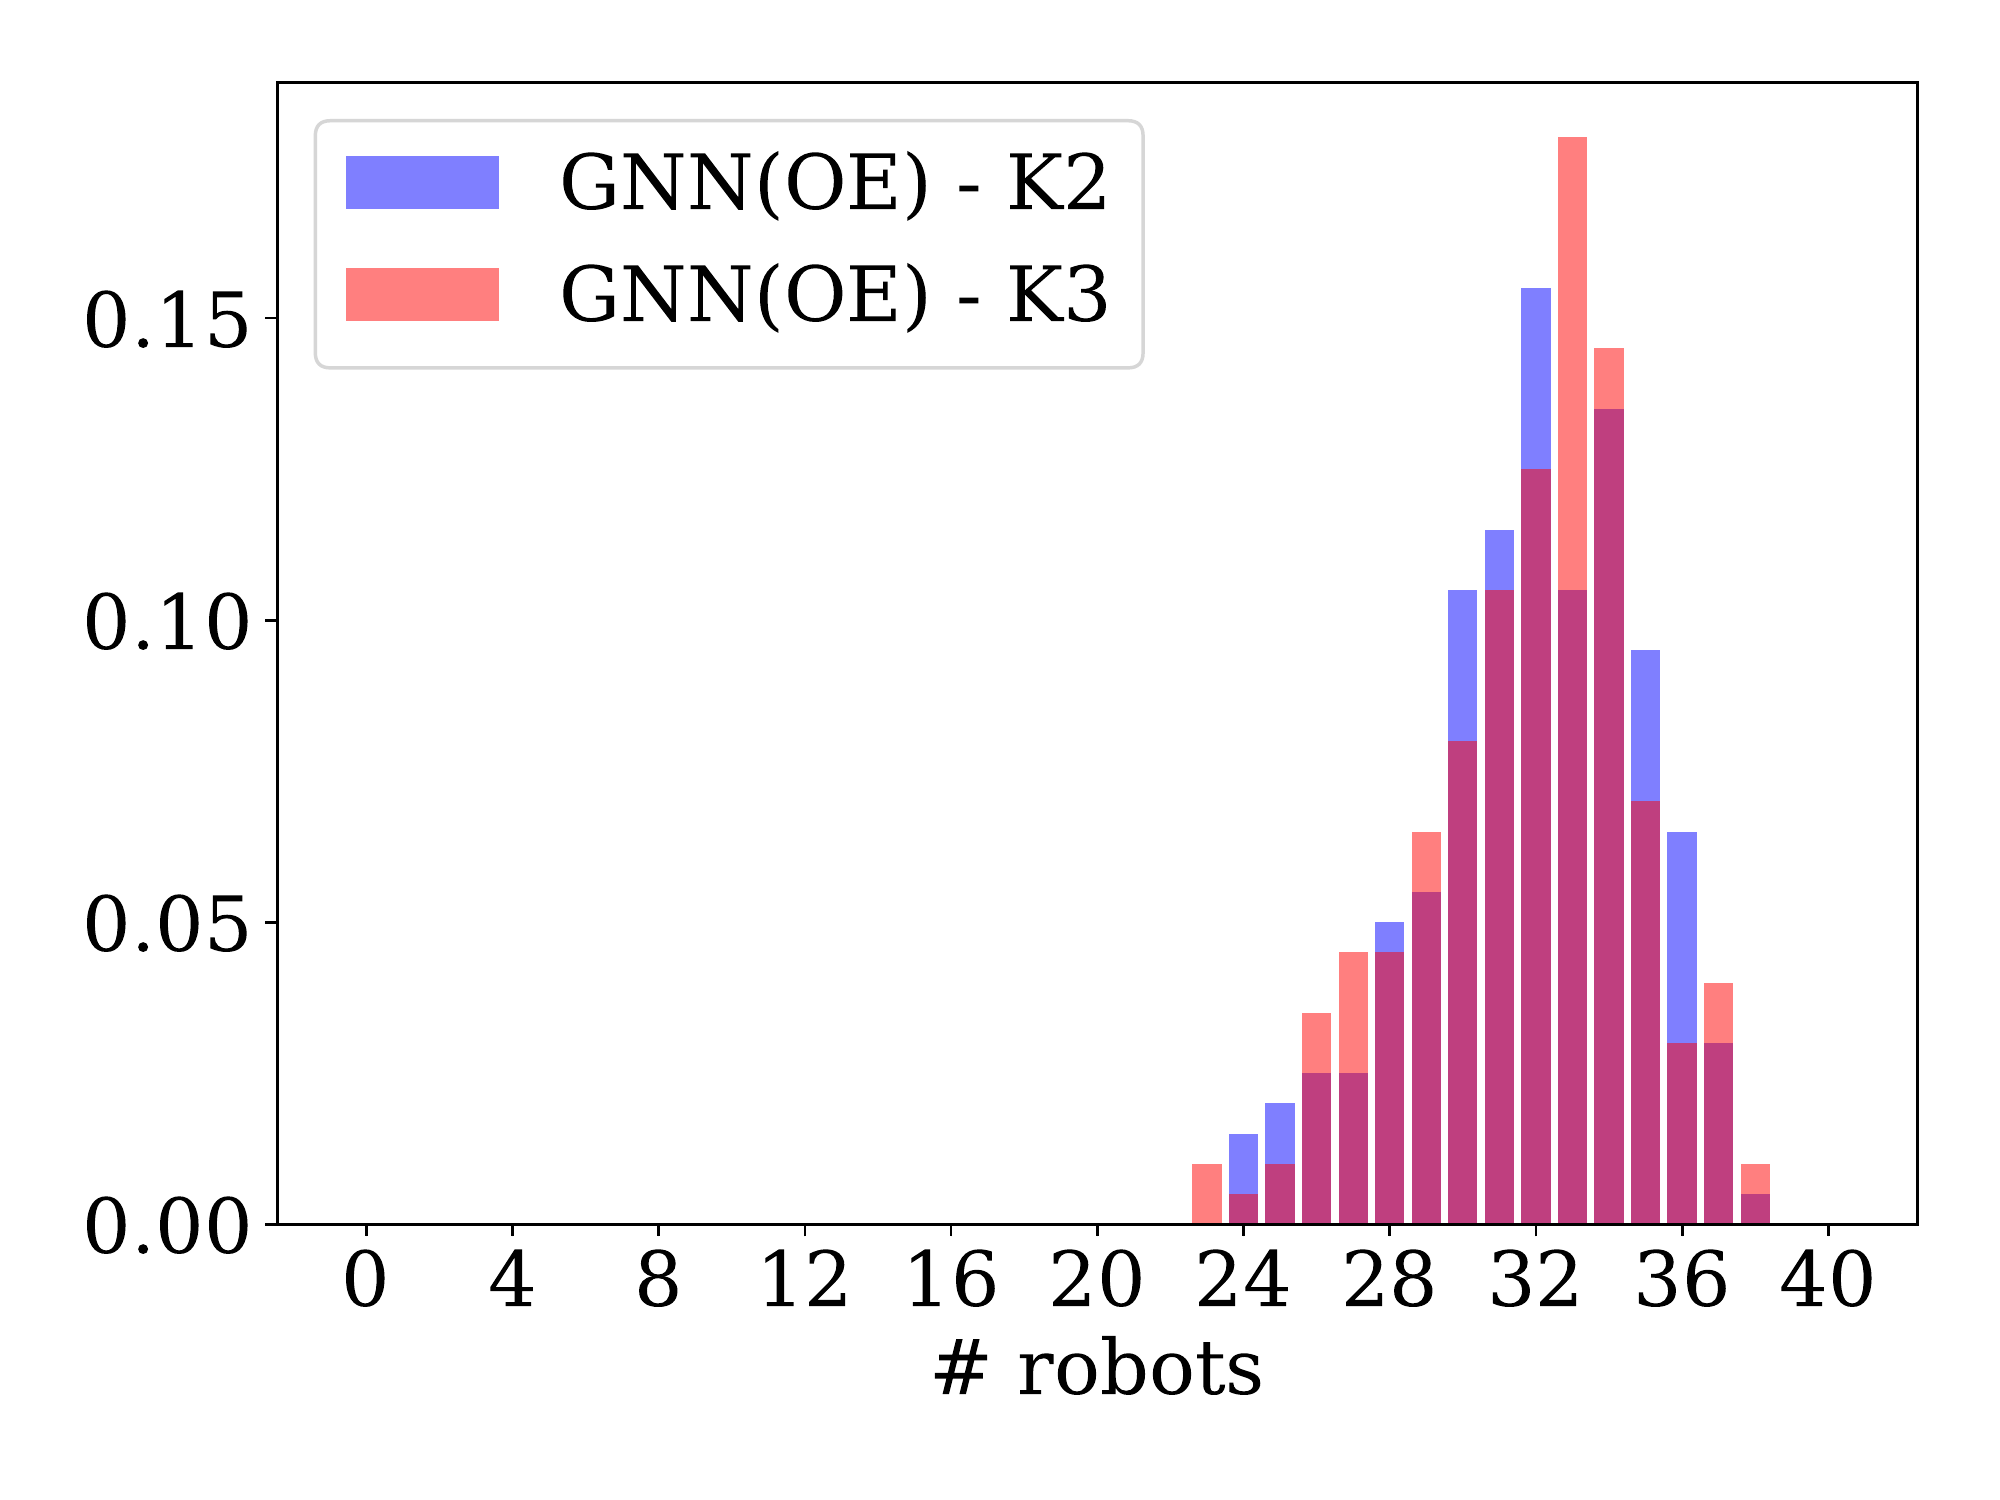}
        \caption{Tested on 40 robots}
    \end{subfigure}
    \caption{\normalfont Histogram of proportion of cases distributed over the number of robots reaching their goal; the network is trained on 10 robots and tested on 20 robots in (a), and tested on 40 robots in (b). Panels (a) and (b) use hop count $K=2$ and $K=3$ with online expert, respectively.}
    \label{fig:results_generalization_impact_K}
\end{figure}
